# Supplementary material for: Interacting line-node semimetal: Proximity effect and spontaneous symmetry breaking
Source: arXiv:1607.07867 ancillary file (2017-07-29)
Supplement: Supplementary file 1 [file LineNode_Supplementary.pdf]

# Supplementary Materials: Interacting line-node semimetal: Proximity effect and spontaneous symmetry breaking

Bitan Roy[1,2]

[1]*Condensed Matter Theory Center and Joint Quantum Institute, University of Maryland, College Park, Maryland 20742-4111, USA*

[2]*Department of Physics and Astronomy, Rice University, Houston, Texas 77005, USA*

The Supplementary Material contains:

1. Minimal representation and no-doubling theorem for three dimensional line-node semimetals,
2. Mean field susceptibility of various orders in a line-node semimetal,
3. Mean field gap equation in the presence of charge-density-wave and antiferromagnet orders,
4. Large $N$ renormalization group analysis, capturing transition into various borken symmetry phases,
5. Correction to anomalous dimensions for various fermion bilinears due to long range Coulomb interaction,
6. Derivation of $Cl(3) \times Cl(3)$ algebra among mass matrices in a line-node semimetal from Clifford algebra,
7. Quasi-particle spectrum inside various superconducting ground states and their symmetries,
8. Quantum critical scaling across a continuous quantum phase transition in the bulk,
9. Details of Hartree-Fock numerical analysis.

## I. MINIMAL REPRESENTATION OF A THREE DIMENSIONAL LINE NODE SEMIMETAL

We first demonstrate the minimal representation for a Dirac-loop and Weyl-loop semimetals. Recall that the tight-binding Hamiltonian for any line-node semimetal in a cubic lattice reads as

$$H_0 = t_1 \sum_{\mathbf{k}} \Psi^\dagger_{\mathbf{k}} \left[\cos(k_x a) + \cos(k_y a) - b\right] \tau_1 \Psi_{\mathbf{k}} + \sum_{\mathbf{k}} \Psi^\dagger_{\mathbf{k}} \left[t_2 (\cos(k_z a) - 1)\tau_1 + t_3 \sin(k_z a)\tau_2\right] \Psi_{\mathbf{k}}, \tag{1}$$

where $a$ is the lattice spacing, as announced in the main part of the paper. For now we do not specify the dimensionality of spinor basis. Two mutually anticommuting matrices $\tau_1$ and $\tau_2$, satisfying the relation $\{\tau_1, \tau_2\} = 0$. The above model supports sharp gapless quasiparticle excitation around an isolated ring in the $k_z = 0$ plane when $|b| < 2$, and the term proportional to $t_2$ plays the role of momentum dependent Wilson mass. Without any loss of generality we choose $\tau_1(\tau_2)$ to be purely real (imaginary).

Let us first focus on a line-node semimetal that remains invariant under the reversal of time. The time-reversal operator $\mathcal{T} = UK$, where $U$ is unitary operator and $K$ is complex conjugation. Thus time-reversal symmetry of the Hamiltonian operator mandates that $\mathcal{T} = K$, with $\mathcal{T}^2 = +1$. Hence, one can realize a isolated nodal ring in the momentum space, arising from hopping of spinless fermions among the nearest-neighbor sites of two interpenetrating sublattices of a cubic lattice, and we can define the spinor basis as $\Psi^\top_{\mathbf{k}} = (c_{A,\mathbf{k}}, c_{B,\mathbf{k}})$. Here, $c_{j,\mathbf{k}}$ is the fermion annihilation operator on sublattice $j = A, B$ with momentum $\mathbf{k}$. Two anticommuting matrices $\tau_1$ and $\tau_2$ can, therefore, be chosen as standard off-diagonal Pauli matrices. Therefore, a Dirac-loop semimetal (DLSM) is devoid of doubling of the number of loops in the momentum space while preserving the $\mathcal{T}$ symmetry, and a two component DLSM can be realized for spinless fermion from a microscopic tight-binding model. This situation is quite different than the one for two and three dimensional Dirac-node semimetals, for which the minimal representaion for Dirac spinor (without the standard doubling due to real spin of fermion) is respectively four and eight [1, 2].

For a time-reversal symmetry breaking Weyl-loop semimetal we can choose $\mathcal{T} = i\tau_2 K$ and the Hamiltonian does not preserve the $\mathcal{T}$ symmetry. Hence, $\mathcal{T}^2 = -1$, and we can define a two component spinor as $\Psi^\top_{\mathbf{k}} = (c_{\uparrow,\mathbf{k}}, c_{\downarrow,\mathbf{k}})$, where $s = \uparrow / \downarrow$ are two projections of spin. Thus an isolated Weyl-loop can be realized in a $\mathcal{T}$ breaking system from spin dependent hopping on a cubic lattice. Two Kramers non-degenerate bands (valence and conduction) touch at each point of such ring in the Brillouin zone. The system is named as Weyl-loop semimetal (WLSM). Therefore,

WLSM as well does not suffer from fermion doubling unlike three dimensional Weyl-node semimetal.

The absence of the third Pauli matrix $\tau_3$ ensures the spectral symmetry of $H_0$, while the inversion symmetry ($\mathcal{P}$), under which $\mathbf{k} \to -\mathbf{k}$ and $\Psi_{\mathbf{k}} \to \tau_1 \Psi_{-\mathbf{k}}$ guarantees that the nodal ring is pinned at the $k_z = 0$ plane.

## II. SUSCEPTIBILITY OF VARIOUS ORDERS

We now display evaluation of susceptibility for various fermionic bilinears or order parameters (OPs) in a DLSM. For a given OP $\Delta_{\mu\nu} = \langle \Psi^\dagger \sigma_\mu \otimes \tau_\nu \Psi \rangle$, the mean field susceptibility (for zero external frequency and mimentum) is given by

$$\chi_{\mu\nu} = -2\ \mathbf{Tr} \int' \frac{dk_r dk_z}{(2\pi)^2} \int_{-\infty}^{\infty} \frac{d\omega}{2\pi} \left[ (\sigma_\mu \otimes \tau_\nu) \frac{i\omega + \hat{H}_0}{\omega^2 + v_r^2 k_r^2 + v_z^2 k_z^2} (\sigma_\mu \otimes \tau_\nu) \frac{i\omega + \hat{H}_0}{\omega^2 + v_r^2 k_r^2 + v_z^2 k_z^2} \right], \tag{2}$$

where $\hat{H}_0 = \sigma_0 \otimes (\tau_1 v_r k_r + \tau_2 v_z k_z)$. Here $\omega$ is the fermionic Matsubara frequency and $\mathbf{Tr}$ is operative over four dimensional matrices. For various choices of $\mu$ and $\nu$ (accept for $\mu = \nu = 0$ for which $\Delta_{00}$ represents the chemical potential), we find

$$\begin{aligned}
\chi_{03} &= \chi_{j3} = \frac{N_f}{\pi^2} \int' \frac{dk_r dk_z}{(2\pi)^2} \frac{1}{\sqrt{v_r^2 k_r^2 + v_z^2 k_z^2}}, \quad \chi_{01} = \chi_{j1} = \frac{N_f}{2\pi^2} \int' \frac{dk_r dk_z}{(2\pi)^2} \left[ \frac{1}{\sqrt{v_r^2 k_r^2 + v_z^2 k_z^2}} + \frac{v_r^2 k_r^2 - v_z^2 k_z^2}{[v_r^2 k_r^2 + v_z^2 k_z^2]^{3/2}} \right], \\
\chi_{02} &= \chi_{j2} = \frac{N_f}{2\pi^2} \int' \frac{dk_r dk_z}{(2\pi)^2} \left[ \frac{1}{\sqrt{v_r^2 k_r^2 + v_z^2 k_z^2}} + \frac{-v_r^2 k_r^2 + v_z^2 k_z^2}{[v_r^2 k_r^2 + v_z^2 k_z^2]^{3/2}} \right], \\
\chi_{j0} &= 8N_f \int' \frac{dk_r dk_z}{(2\pi)^2} \int_{-\infty}^{\infty} \frac{d\omega}{2\pi} \frac{\omega^2 - \left( v_r^2 k_r^2 + v_z^2 k_z^2 \right)}{\left( \omega^2 + v_r^2 k_r^2 + v_z^2 k_z^2 \right)^2} = 0,
\end{aligned} \tag{3}$$

after completing the integral over Matsubara frequency $\omega$, for $j = 1, 2, 3$. Here $N_f$ represents the number of four component spinor. The integral over spatial components of momentum is restricted within $0 < k_r < \Lambda$ and $0 < |k_z| < \Lambda$. Thus momentum integral can easily be performed by introducing a new set of variable as $v_r k_r = vk \sin\theta$ and $v_z k_z = vk \cos\theta$, and the integrals over newly introduced variables are restricted within the region $0 < k < \Lambda$ and $0 \leq \theta \leq \pi$. Finally we obtain

$$\chi_{03} = \chi_{j3} = \left[ \frac{vN_f}{\pi v_r v_z} \right] \Lambda, \quad \chi_{01} = \chi_{02} = \chi_{j1} = \chi_{j2} = \left[ \frac{vN_f}{\pi v_r v_z} \right] \frac{\Lambda}{2}, \quad \chi_{j0} = 0. \tag{4}$$

We have quoted this result in the main part of the paper, with $f(v_r, v_z) = (vN_f)/(\pi v_r v_z)$. The critical couplign for any such ordering $g_c^{\mu\nu} \propto \chi_{\mu\nu}^{-1}$.

## III. MEAN-FIELD GAP EQUATION

We here demonstrate the derivation and solution of the mean field gap equation, announced in the main part of the paper, in the presence of charge-density-wave (CDW) and antiferromagnet (AF) orderings. For concreteness, we also display the calculation for the self-consistent solution for the CDW order parameter ($\Delta_3$). Similar calculation can also be carried out for the AF order parameter ($|\vec{\Delta}_3|$). The energy spectrum in the presence of these two order parameters (OPs) reads as

$$E_{\mathbf{k},\sigma} \left( \Delta_3, |\vec{\Delta}_3| \right) = \pm \sqrt{ \left( \frac{k_\perp^2 - k_F^2}{2m} \right)^2 + v_z^2 k_z^2 + \Delta_3^2 + |\vec{\Delta}_3|^2 + 2\sigma \Delta_3 |\vec{\Delta}_3| }, \tag{5}$$

for $\sigma = \pm$. The corresponding free energy in the presence of these two orderings is

$$F \left( \Delta_3, |\vec{\Delta}_3| \right) = \frac{\Delta_3^2}{2g_C} + \frac{|\vec{\Delta}_3|^2}{2g_{AF}} - 2 \sum_{\sigma=\pm} \int' \frac{d^3\mathbf{k}}{(2\pi)^3} E_{\mathbf{k},\sigma} \left( \Delta_3, |\vec{\Delta}_3| \right), \tag{6}$$

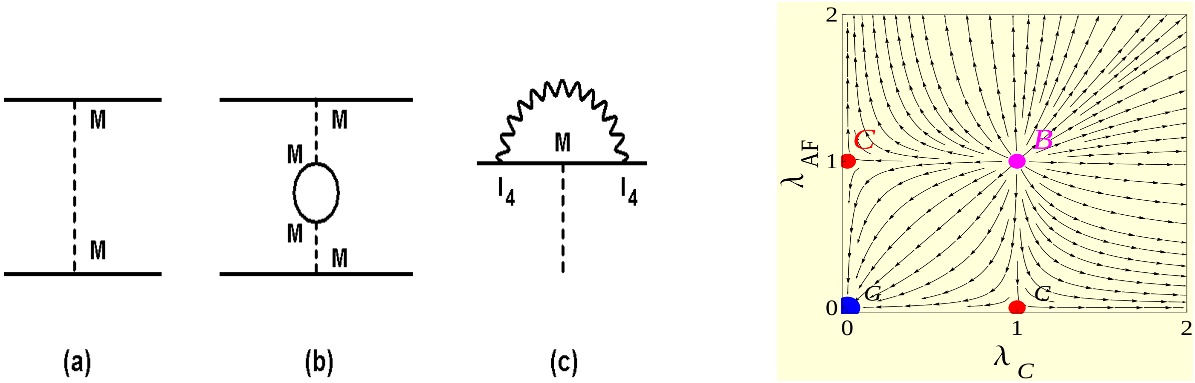


Figure 1: Left: Feynman diagram (a) represents a bare four-fermion interaction coupling ($g$). Diagram (b) is the only relevant one-loop diagram, giving rise to renormalization of bare interaction vertex, in the large $N_f$ limit. Here $M$ is a four component Hermitian matrix, and solid lines represents fermions. (c) Leading order correction to the anomalous dimension of a fermion bilinear $\Psi^\dagger M \Psi$ due to the long range tail of the Coulomb interaction (represented by the wavy line). Here $I_4$ is the four dimensional identity matrix. Right: RG flow diagram in $(\lambda_C, \lambda_{AF})$ plane for $\epsilon = 1$. Here, the blue dot represents fully stable Gaussian fixed point representing a DLSM, while the red dots stand for quantum critical points. These two quantum critical points controls the continuous transition from a DLSM to CDW (one residing on $\lambda_{AF} = 0$ axis) and AF (one residing on $\lambda_C = 0$ axis) phases. The magneta dot is the bicritical point, controling the first order transition between AF and CDW phases.

where $g_C = (6V - U)/8$ and $g_{AF} = U/8$ are the local four fermion interaction that respectively supports the CDW and AF orders. Here, $U$ and $V$ are the strength of onsite and nearest-neighbor repulsions.

Let us first focus on the CDW ordering seprately, and set $|\vec{\Delta}_3| = 0$. Then minimizing the free energy we arrive at the following mean field gap equation (after taking $2g_C \to g_C$)

$$\frac{1}{g_C} = \int \frac{d^3\mathbf{k}}{(2\pi)^3} \frac{1}{E_{\mathbf{k}}(\Delta_3)} \;\Rightarrow \frac{1}{g_C} = \int_0^{E_\Lambda} d\varepsilon \frac{\varrho(\varepsilon)}{\sqrt{\varepsilon^2 + \Delta_3^2}} \;\Rightarrow \frac{1}{g_C} - \int_0^{E_\Lambda} d\varepsilon = \int_0^{E_\Lambda} d\varepsilon \left[ \frac{\varrho(\varepsilon)}{\sqrt{\varepsilon^2 + \Delta_3^2}} - 1 \right], \tag{7}$$

where $\varrho(\varepsilon) \sim |\varepsilon|$ is the density of states in a line-node semimetal and $E_\Lambda$ is the high energy cutoff up to which the dispersion is linear. In term of a dimensionless parameter $\delta_C$, defined as $\delta_C = [1/g_C^\ast - 1/g_C]\, E_\Lambda^{-1}$ the solution of the above gap equation is

$$\delta_C = 1 + m_C - \sqrt{1 + m_C^2}, \tag{8}$$

where $m_C = \Delta_3/E_\Lambda$ is the dimensioless CDW OP, as shown in the main part of the paper. The parameter $\delta_C$ measures the distance from the nonuniversal strength of critical nearest-neighbir interaction ($g_C^\ast$) for the CDW ordering. Similar self consistent solution can also be found for the AF OP in the absence of CDW OP, i.e. when $\Delta_3 = 0$.

The coupled gap equations in the presence of these two orderings read as

$$\frac{1}{g_C} = 2 \sum_{\sigma=\pm} \int' \frac{d^3\mathbf{k}}{(2\pi)^3} \frac{[1 + 2\sigma \Delta_3 |\vec{\Delta}_3|^{-1}]}{E_{\mathbf{k},\sigma}\left(\Delta_3, |\vec{\Delta}_3|\right)}, \quad \frac{1}{g_{AF}} = 2 \sum_{\sigma=\pm} \int' \frac{d^3\mathbf{k}}{(2\pi)^3} \frac{[1 + 2\sigma |\vec{\Delta}_3| \Delta_3^{-1}]}{E_{\mathbf{k},\sigma}\left(\Delta_3, |\vec{\Delta}_3|\right)}. \tag{9}$$

We numerically solve these two coupled gap equations in “Mathematica” and minimize the free energy to obatin the phase diagram, displaed as Fig. 1 (a) in the main part of the paper.

## IV. LARGE-N RENORMALIZATION GROUP CALCULATION

To anchor the nature of the QPTs from a DLSM to BSPs and between two distinct BSPs, we perform a renormalization group (RG) calculation. The Euclidean action for minimal interacting model reads as

$$S = \int \frac{d\omega}{2\pi} \int' d^{1+\epsilon}\mathbf{k} \int d\theta \; \Psi_\alpha^\dagger \left[-i\omega + H_0\right] \Psi_\alpha - \sum_{j=C,AF} g_j \int \prod_{i=1}^{3} \frac{d\omega_i}{2\pi} \int' d^{1+\epsilon}\mathbf{k}_i \int d\theta_i \, \left(\Psi_{1+2-3}^\dagger M_j \Psi_1\right) \, \left(\Psi_3^\dagger M_j \Psi_2\right) \tag{10}$$

where $\alpha \equiv (\omega, \mathbf{k}, \theta)$, $H_0 = \Gamma_1 v_r k_r + \Gamma_2 v_z k_z$, $M_C = \sigma_0 \otimes \tau_3$ and $M_{AF} = \vec{\sigma} \otimes \tau_3$. Fermionic field $\Psi_i$ $(i = 1, \cdots, 4)$ is a function of $\alpha_i \equiv (\omega_i, \mathbf{k}_i, \theta_i)$. The integral over momentum is restricted up to an ultraviolet cut-off $\Lambda$. The scaling dimension of four-femrion interaction is $[g_j] = 1 - d_c$, where $d_c$ is the *co-dimension.* For a three dimensional DLSM is $d_c = 2$ [3, 4]. Hence $[g_j] = -1$ and sufficiently weak short-range interaction is an *irrelevant* perturbation in a DLSM and the potential breakdown of the noninteracting fixed point at strong interaction can be demonstrated via a RG calcualtion, controlled via a simultaneous $1/N_f$ and $\epsilon$-expansions about a lower critical co-dimension $d_c^\ast = 1$ (representing a Fermi surface), where $N_f$ is the number of four-component spinor and $\epsilon = d_c - 1$.

We now present some essential details of the renormalization group calculation performed using simultaneous large $N_f$ and $\epsilon$-expansion in a DLSM. In the $N_f \to \infty$ limit only diagram (b) from Fig. 1 contributes to the renormalization of the bare interaction coupling. The contribution from this diagram reads as

$$(1,\mathrm{b}) = -2 g_j^2 \, \mathbf{Tr} \int' \frac{dk_r dk_z}{(2\pi)^2} \int_{-\infty}^{\infty} \frac{d\omega}{2\pi} \left[ M_j \, \frac{i\omega + \hat{H}_0}{\omega^2 + v_r^2 k_r^2 + v_z^2 k_z^2} \, M_j \, \frac{i\omega + \hat{H}_0}{\omega^2 + v_r^2 k_r^2 + v_z^2 k_z^2} \right], \tag{11}$$

where $M_j = \sigma_0 \otimes \tau_3$ and $\vec{\sigma} \otimes \tau_3$ respectively for $j = C, AF$. After completing the frequency integral we obtain

$$(1,\mathrm{b}) = \frac{g_j^2 N_f}{\pi^2} \int' dk_r dk_z \, \frac{1}{\sqrt{v_r^2 k_r^2 + v_z^2 k_z^2}} = \frac{g_j^2 N_f \Lambda^\epsilon}{\pi v} = g_j \lambda_j, \tag{12}$$

after integrating over the Wilsonian shell $\Lambda e^{-l} < k_r < \Lambda$ and $\Lambda e^{-l} < |k_z| < \Lambda$, where $\lambda_j = \frac{g_j N_f \Lambda^\epsilon}{\pi v}$ is the dimensionless coupling constant. Upon performing subsequent rescale according to $\omega \to e^{-l}\omega$, $k_{r/z} \to e^{-l} k_{r/z}$, $\Psi \to e^{(3+\epsilon)l/2}\Psi$, we arrive at the flow equations

$$\frac{d\lambda_C}{dl} = -\epsilon \lambda_C + \lambda_C^2, \; \frac{d\lambda_{AF}}{dl} = -\epsilon \lambda_{AF} + \lambda_{AF}^2, \tag{13}$$

in $N_f \to \infty$ limit. The fact that dimensionless coupling constant $\lambda_j \sim \Lambda^\epsilon g_j$, ensures that our RG analysis is controlled in the framework of $\epsilon$-expansion, performed within Wilsonian shell integration scheme.

All together, the above flow equations support four fixed point: (i) $(\lambda_C, \lambda_{AF}) = (0,0)$, (ii) $(\lambda_C, \lambda_{AF}) = (\epsilon, 0)$, (iii) $(\lambda_C, \lambda_{AF}) = (0, \epsilon)$ and (iv) $(\lambda_C, \lambda_{AF}) = (\epsilon, \epsilon)$, as shown in Fig. 1 (Right) (after setting $\epsilon = 1$). The first one is a fully stable Gaussian fixed point, representing a stable DLSM for sufficiently weak interactions. The second and third ones are quantum critical points (QCPs) with only one unstable direction, respectively describing the transition to CDW and AF phases for sufficiently strong $\lambda_C \sim V$ and $\lambda_{AF} \sim U$. The last one is a bicritical point with two unstable directions, indicating a first order transition between these two distinct BSPs. The corresponding phase diagram in the $(V/U_c, U/U_c)$ plane is shown in Fig. 1 (Right), where $U_c$ is the nonuniversal critical strengths of onsite repulsions for AF orderings.

Similar scaling analysis and RG calculation indicates the onset of a $\mathcal{P}$, $\mathcal{T}$-odd magnetic ordering $(\Delta_M)$ through a continuous QPT for sufficiently strong Hubbard interaction in WLSM. The interacting Hamiltonian is $H_{int} = g_F (\Psi^\dagger \sigma_3 \Psi)^2$, where $\Psi$ is now a two-component spinor. The possible continuous phase transition is captured by the RG flow equation

$$\frac{d\lambda_F}{dl} = -\epsilon \lambda_F + \frac{1}{2} \lambda_F^2, \tag{14}$$

where $\lambda_F$ is the dimensionless four-fermion coupling defined as $\lambda_F = g_F \Lambda^\epsilon N_f/(\pi v)$ and $N_f$ is the number of two-component spinor. However, it should be noted perturbative RG flow equation for a single two-component Dirac/Weyl fermion vanishes at least to the order $g_F^3$ [5]. However, this model is expected to support a quantum phase transition at strong coupling [6].

## V. CORRECTION TO ANOMALOUS DIMENSION OF VARIOUS FERMION BILINEARS DUE TO LONG RANGE COULOMB INTERACTION

We now discuss the correction to the anomalous dimension of various fermion bilinears, represented as $\Psi^\dagger M \Psi$, where $M$ is a four dimensional Hermitian matrix due to long range Coulomb interaction in a DLSM. Such correction

to the anomalous dimension arises from diagram (c) in Fig. 1. Contribution from this diagram reads as

$$\chi^C_{\mu\nu} = -2e^2 \int' \frac{dk_r dk_z}{(2\pi)^2} \int_{-\infty}^{\infty} \frac{d\omega}{2\pi} \frac{i\omega + \hat{H}_0}{\omega^2 + v_r^2 k_r^2 + v_z^2 k_z^2} \; (\sigma_\mu \otimes \tau_\nu) \; \frac{i\omega + \hat{H}_0}{\omega^2 + v_r^2 k_r^2 + v_z^2 k_z^2} \quad \frac{1}{k_r^2 + k_z^2}, \tag{15}$$

where $e$ is the electronic charge. Upon completing the integral over the Matsubara frequency we find

$$\chi^C_{03} = \chi^C_{j3} = \frac{e^2}{4\pi^2 v_r} \int' \frac{dk_r dk_z}{(k_r^2 + \eta^2 k_z^2)^{1/2}} \quad \frac{1}{k_r^2 + k_z^2}, \quad \chi^C_{0j} = 0,$$
$$\chi^C_{01} = \chi^C_{02} = \chi^C_{j1} = \chi^C_{j2} = \frac{e^2}{8\pi^2 v_r} \int' \frac{dk_r dk_z}{(k_r^2 + \eta^2 k_z^2)^{1/2}} \quad \frac{1}{k_r^2 + k_z^2}, \tag{16}$$

where $\eta = v_z/v_r$. Next we integrate out a thin Wolsonian shell with $\Lambda e^{-l} < q_r < \Lambda$ and $\Lambda e^{-l} < |q_z| < \Lambda$, to capture the enhancement of anomalous dimension. We find

$$\chi^C_{03} = \chi^C_{j3} = \frac{\alpha_r}{\Lambda} \, F(\eta) \, l \quad \text{and} \quad \chi^C_{01} = \chi^C_{02} = \chi^C_{j1} = \chi^C_{j2} = \frac{1}{2} \frac{\alpha_r}{\Lambda} \, F(\eta) \, l, \tag{17}$$

where $\alpha_r = e^2/(4\pi^2 v_r)$ can be considered as the fine structure constant along the radial direction. The function

$$F(\eta) = \mathrm{E}_k(1-\eta^2) + \frac{\mathrm{E}_k(1-\eta^{-2})}{\eta}, \tag{18}$$

where $\mathrm{E}_k$ is the elliptic function of first kind. Therefore, mass orderings receive largest boost through the enhancement of anomalous dimension due to the long range tail of the Coulomb interaction in a DLSM, as announced in the main part of the paper. Similar conclusion can readily be generalized for WLSM, suggesting that a ferromagnetic order receives largest boost in anomalous dimension from long range tail of the Coulomb interaction.

## VI. DERIVATION OF INTERNAL ALGEBRA AMONG MASSES IN A DIRAC-LOOP SEMIMETAL

We here provide a proof of $Cl(3) \times Cl(3)$ algebra among various mass matrices (representing two insulators and one superconductor) in a DLSM. Our derivation is based on Clifford algebra and does not rely on specific microscopic details of the model. Let us define a Nambu-doubled spinor as $\Psi = (\Psi_p, \Psi_h)^\top$ so that the effective Hamiltonian describing low energy excitations in a DLSM assumes the form

$$H_{DL}(\mathbf{k}) = H_0(\mathbf{k}) \oplus \left[ -H_0^\top(-\mathbf{k}) \right], \tag{19}$$

where

$$H_0(\mathbf{k}) = \sum_{j=1,2} \alpha_j \, d_j(\mathbf{k}), \quad \text{and} \quad d_1(\mathbf{k}) = \frac{k_x^2 + k_y^2 - k_F^2}{2m}, \; d_2(\mathbf{k}) = v_z k_z. \tag{20}$$

Here $\alpha_1$ and $\alpha_2$ are two mutually anticommuting four component Hermitian matrices. Next we wish to find all the Hermitian eight dimensional matrices ($M$s) that anticommute with $H_{DL}(\mathbf{k})$, such that $m = \langle \Psi^\dagger M \Psi \rangle \neq 0$. Therefore, $M$s represent mass matrices. Such condition is satisfied only when

$$M = -\left(\sigma_1 \otimes \mathbb{I}_4\right) \, M^\top \, \left(\sigma_1 \otimes \mathbb{I}_4\right), \tag{21}$$

where $\mathbb{I}_4$ is a four dimensional identity matrix. There exists a unitary matrix $U = U_2 \otimes \mathbb{I}_4$ such that $\tilde{M} = -\tilde{M}^\top$, where $\tilde{M} = U M U^\dagger$ and

$$U_2 = \sqrt{\pm i} \; e^{i\frac{\pi}{4}\sigma_3} \; e^{i\frac{\pi}{4}\sigma_2} \; e^{i\left(\frac{\pi}{4}-\phi\right)\sigma_3}. \tag{22}$$

Therefore, after the unitary transformation all mass matrices are purely *imaginary* [7].

Let us now write two mutually anticommuting four dimensional matrices, appearing in $H_0(\mathbf{k})$ as

$$\alpha_j = \Re(\alpha_j) + i \, \Im(\alpha_j), \tag{23}$$

| Pairing | available in | Spin tructure | Spectrum |
|---|---|---|---|
| $\Delta_0$ | DLSM | singlet | $E_\alpha(\mathbf{k}) = \pm \left[d_1^2(\mathbf{k}) + d_2^2(\mathbf{k}) + \Delta_0^2 + \mu^2 - 2\alpha\sqrt{\mu^2(d_1^2(\mathbf{k}) + d_2^2(\mathbf{k})) + \Delta_0^2 d_2^2(\mathbf{k})}\right]^{1/2}$ |
| $\Delta_s$ | DLSM | singlet | $E_\alpha(\mathbf{k}) = \pm \left[\left(\sqrt{d_1^2(\mathbf{k}) + d_2^2(\mathbf{k})} - \alpha\mu\right)^2 + \Delta_s^2\right]^{1/2}$ |
| $\Delta_2$ | DLSM | singlet | $E_\alpha(\mathbf{k}) = \pm \left[d_1^2(\mathbf{k}) + d_2^2(\mathbf{k}) + \Delta_0^2 + \mu^2 - 2\alpha\sqrt{(\mu^2 + \Delta_2^2)[d_1^2(\mathbf{k}) + d_2^2(\mathbf{k})]}\right]^{1/2}$ |
| $\Delta_t$ | DLSM | triplet | $E_\alpha(\mathbf{k}) = \pm \left[d_1^2(\mathbf{k}) + d_2^2(\mathbf{k}) + \Delta_t^2 + \mu^2 - 2\alpha\sqrt{\mu^2(d_1^2(\mathbf{k}) + d_2^2(\mathbf{k})) + \Delta_t^2 d_1^2(\mathbf{k})}\right]^{1/2}$ |
| $\Delta_W$ | WLSM | singlet | $E_\alpha(\mathbf{k}) = \pm \left[d_1^2(\mathbf{k}) + d_2^2(\mathbf{k}) + \Delta_W^2 + \mu^2 - 2\alpha\sqrt{\mu^2(d_1^2(\mathbf{k}) + d_2^2(\mathbf{k})) + \Delta_W^2 d_2^2(\mathbf{k})}\right]^{1/2}$ |

Table I: Quasiparticle spectrum within the mean field approximation in the presence of various local pairing in DLSM and WLSM, where $\alpha = \pm$. Each branch is two fold Kramers degenerate in DLSM, while Kramers degeneracy is absent in WLSM.

for $j = 1, 2$. After such decomposition the kinetic energy of a DLSM assumes the form

$$H_{DL}(\mathbf{k}) = [\sigma_3 \otimes \Re(\alpha_1) + i\sigma_0 \otimes \Im(\alpha_1)]\, d_1(\mathbf{k}) + [\sigma_0 \otimes \Re(\alpha_2) + i\sigma_3 \otimes \Im(\alpha_2)]\, d_2(\mathbf{k}). \tag{24}$$

Since $U_2 \sigma_3 U^\dagger = \sigma_2$, after the unitary transformation with $U$ the kinetic energy becomes

$$\tilde{H}_{DL}(\mathbf{k}) = [\sigma_2 \otimes \Re(\alpha_1) + i\sigma_0 \otimes \Im(\alpha_1)]\, d_1(\mathbf{k}) + [\sigma_0 \otimes \Re(\alpha_2) + i\sigma_2 \otimes \Im(\alpha_2)]\, d_2(\mathbf{k}) = \tilde{\Gamma}_1 d_1(\mathbf{k}) + \tilde{\Gamma}_2 d_2(\mathbf{k}). \tag{25}$$

Thus, $\tilde{\Gamma}_1$ and $\tilde{\Gamma}_2$ are respectively mutually anticommuting, but purely imaginary and real eight dimensional Hermitian matrices. We are after find all purely imaginary matrices ($\tilde{M}$) that anticommutes with $\tilde{\Gamma}_1$ and $\tilde{\Gamma}_2$. Since, $i\tilde{\Gamma}_1$ and $i\tilde{M}$ are purely imaginary and square to $-1$, while $\tilde{\Gamma}_2$ is purely real and squares to $+1$, we seek to know maximal number of $q$ so that for $p \geq 1$, the dimensionality of real matrices is eight and together they close $C(p, q)$ algebra. Notice that $C(p, q)$ Clifford algebra is defined by a set of $p + q$ mutually anticommuting matrices, among which $p$ of them squares to $+1$, while $q$ of them squares to $-1$. The answer is $q = 4$ and $p = 1$ [8]. Thus maximal number of mutually anticommuting matrices is 5, and we define a set of such five matrice as $\{R, I_1, I_2, I_3, I_4\}$, where $R$ is real and $I_j$s are imaginary for $j = 1, \cdots, 4$. Two of those five matrices, say $R$ and $I_1$, can be used to define the kinetic energy. Therefore, $I_2, I_3$ and $I_4$ represents three mass matrices that together close a $Cl(3)$ algebra.

The Clifford algebra $C(1, 4)$ follows the quaternionic representation that supports *three* real Casimir operators, $K_j$ for $j = 1, 2, 3$, besides the standard identity matrix. The Casimir operators satisfy the quaternionic algebra

$$K_i K_j = -\delta_{ij} + \epsilon_{ijk} K_k, \tag{26}$$

where $\delta_{ij}$ is the Kroneker delta function. From the casimir operators we can define imaginary matrices $E_j = iK_j$ for $j = 1, 2, 3$ and $E_j$s satisfy the $SU(2)$ algebra [7]. Notice that $E_j$s are purely imaginary Hermitian matrices that commute with $H_{DL}(\mathbf{k})$. From these three matrices we can define yet another set of three mutually anticommuting matrices $M'_j = iE_j R I_1$ that together close a $Cl(3)$ algebra and also anticummute with $H_{DL}(\mathbf{k})$. Hence, there are all together six purely imaginary matrices (thus mass) that anticommute with $H_{DL}(\mathbf{k})$ and they can be arranged into two sets according to

$$\{I_2, I_3, I_4\} \quad \text{and} \quad \{M'_1, M'_2, M'_3\}$$

that close a $Cl(3) \times Cl(3)$ algebra, as we announced in the main part of the paper.

## VII. QUASIPARTICLE SPECTRUM IN THE PRESENCE OF PARINGS

Finally we discuss the quasipartile spectrum when pairing orders develop in a DLSM and WLSM. As discussed in the main part of the paper, a DLSM supports a fully gapped $s$-wave pairing. DLSM also supports various other singlet and triplet pairings that does not led to fully gapped quasiparticle spectrum. The effective single particle Hamiltonian in the presence of all possible local pairings in DLSM reads as

$$H_{SC}^{DLSM} = (\eta_1 \cos\phi + \eta_2 \sin\phi) \otimes (\Delta_0 \Gamma_0 + \Delta_s \Gamma_1 + \Delta_2 \Gamma_2 + \Delta_t\, [\vec{\sigma} \otimes \tau_3]), \tag{27}$$

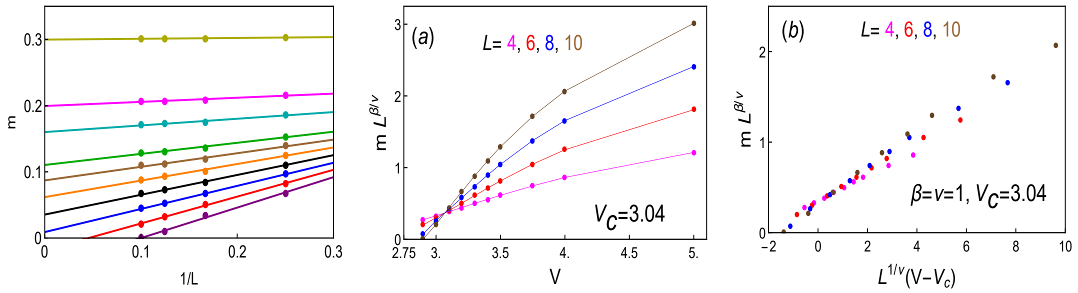


(a) (b) (c)

Figure 2: (a) Scaling of self-consistent solution of charge-density-wave (CDW) order parameter (OP), $m = \Delta_{03}/t$, in the presence of periodic boundary in all three direction as a function of $1/L$, where $L$ is the system size in the $z$-direction, while system size in the $x$ and $y$ direction is always $L_x = L_y = 10$. In this panel the strengths of nearest-neighbor (NN) repulsion are $V/t = 2.9, 3.0, 3.1, 3.2, 3.3, 3.4, 3.5, 3.75, 4.0, 5.0$ from bottom to top. (b) the CDW OP in various systems (with linear dimension $L$ along $z$ direction) cross at $V = 3.04$ when we compare $mL^{\beta/\nu}$ vs. $V$, suggesting critical strength of NN repulsion for CDW ordering in the bulk is $V_c = 3.04$. We here set $\beta = 1$ and $\nu = 1$, the large-N values [see Eq. (31)]. (c) A good quality data collapse is obtained when we compare $mL^{\beta/\nu}$ vs. $L^{1/\nu}(V - V_c)$, with $V_c = 3.04$, strongly sugegsting a second order or continuous quantum phase transition from a three dimensional line-node semimetal to a CDW phase at finite strength of NN interaction.

where $\phi$ is the superconducting phase. On the other hand, a WLSM supports only one local pairing and in the presence of such local pairing effective single particle Hamiltonian is given by

$$H^{WLSM}_{SC} = (\eta_1 \cos\phi + \eta_2 \sin\phi) \otimes (\Delta_W \tau_0)\,. \tag{28}$$

Quasiparticle spectrum in the presence of these pairings is shown in Table I.

In the presence of the singlet pairing [one with the amplitude $\Delta_0$ in Eq. (27)] the spectrum of BdG fermions supports a pair of nodal rings at $k_z = \pm\sqrt{\Delta_0^2 + \mu^2}/v_z$, symmetrically placed about the $k_z = 0$ plane, with its radius being identical to the one in the normal state $k_\perp = k_F$. Consequently, a surface perpendicular to the (0,0,1) directions supports two degenerate circular flat bands of Andreev bound state with radius $k_F$ (drumhead surface states). With increasing chemical potential ($\mu$) or lowering the temperature below $T_c$, pairing amplitude increases monotonically and two thermal LNSM separate further in the reciprocal space.

With an underlying singlet $s$-wave pairing (with amplitude $\Delta_s$) the quasiparticle spectrum is always fully gapped. Such singlet pairing thus represents a Majorana mass for nodal quasiparticles in a DLSM.

The triplet pairing [one with amplitude $\Delta_t$ in Eq. (27)] also supports two nodal ring in the paired phase. However, they are located in the $k_z = 0$ plane, with radii $k^{\pm}_{\perp} = [k_F^2 \pm 2m\sqrt{\Delta_0^2 + \mu^2}]^{1/2}$. The surface Andreev bound state perpendicualr to (0,0,1) direction is comprised of two flat bands, representing the shadows of bulk line nodes. Thus, as the temperature is gradually lowered below the transition temperature ($T_c$) or the chemical potential is gradually increased, the radius of one ring increases, while that for the other ring decreases continuously.

The remaining singlet pairing in DLSM [one with amplitude $\Delta_2$ in Eq. (27)] gives rise to *four* nodal rings, discussed above. Since the condensation energy gain in the presence of four nodal rings are much less than that in the presence of a fully gapped pairing or nodal pairing that supports two thermal LNSM, we believe that such singlet pairing is energetically inferior.

The only local pairing in a WLSM produces a pair of nodal rings located at $k_z = \pm\sqrt{\Delta_W^2 + \mu^2}/v_z$ planes and their radii $k_\perp = k_F$ are identical. Thus with increasing $\mu$ or decreasing temperature below $T_c$, separation of two rings increases.

Appearance of any nodal superconductor (supporting thermal LNSM inside the ordered phase) at low temperatures can be detected from the measurement of specific heat ($C_v$), for example. Assuming that the pairing takes place in the vicinity of the Fermi surface, we expect $C_v/T$ to be roughly constant, at least when temperature $T \ll E_F/k_B$ but $T > T_c$, where $E_F$ is the Fermi energy. Inside the superconducting phase ($T < T_c$) $C_v \sim T^2$,

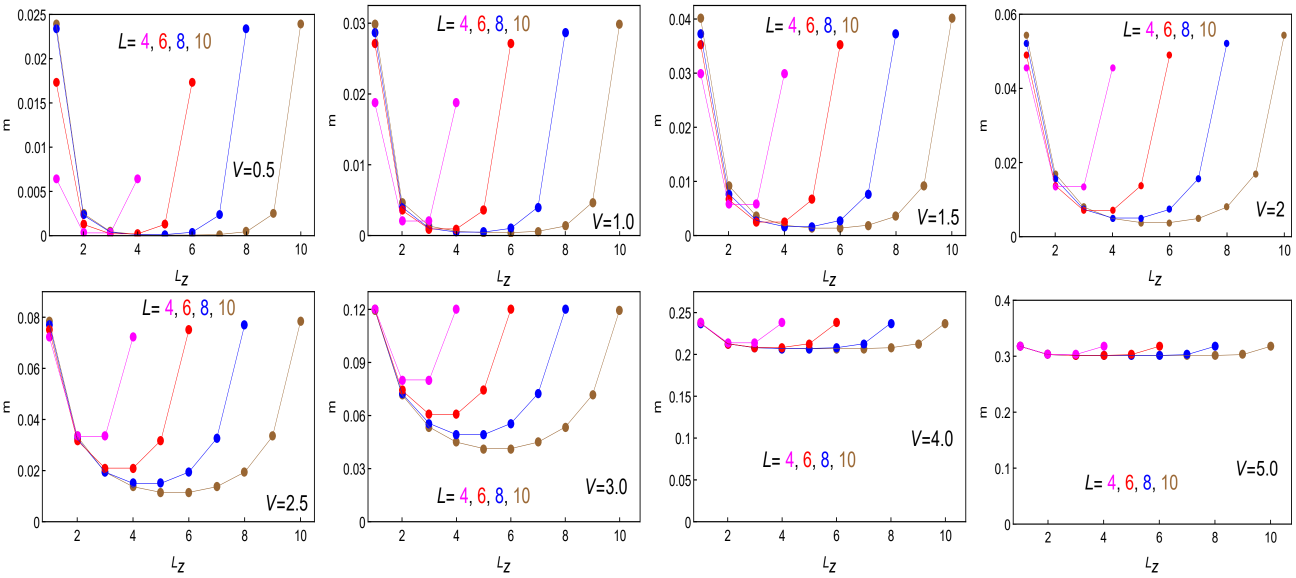


Figure 3: Self consistent solution of the charge-density-wave (CDW) order-parameter for subcritical ($V < V_c = 3.04$) and above critical strength of nearest-neighbor (NN) repulsion (quoted in each subfigrue) in system with various linear dimension along $z$ direction ($L$, quoted in each subfigure), strongly supporting the scenario of proximity induced ordering in the bulk due to drumhead shaped flat surface states. $L_z$ is the layer index in the $z$ direction, along which we implement open boundary.

yielding $C_v/T \sim T$ due to linear density of states arising from gapless BdG quasiparticles residing around the nodal rings. Since, $\varrho(\varepsilon) \sim |\varepsilon|$, ballistic BdG fermion becomes unstable toward the formation of a diffusive Majorana metal for infinitesimal amount of impurity [9, 10]. Thus, inside the paired state once again $C_v/T$ becomes constant as $T \to 0$.

## VIII. QUANTUM CRITICAL SCALING

We here demonstrate the universal scaling of a mass order [such as charge-density-wave (CDW) and anti-ferromagnet (AF)] across a continuous quantum phase transition driven by short-range component of the Coulomb interaction. For concreteness, we here focus only on CDW ordering, which can be driven by nearest-neighbor (NN) repulsion ($V$). A similar scaling theory can also be found for AF ordering, which on the other hand, is supported by onsite repulsion. By definition,

$$m \sim \left| \frac{V - V_c}{V_c} \right|^{\beta} \equiv |\delta|^{\beta}, \tag{29}$$

where $m = \Delta_{03}/t$ is the dimensionless CDW order parameter, and $V$ and $V_c$ (critical strength of NN interaction for CDW ordering) are also measured in units of $t$. The order parameter exponent $\beta$ is related to the correlattion length exponent $\nu$ according to

$$\frac{\beta}{\nu} = \frac{1}{2} \left[ d + z - 2 + \eta \right], \tag{30}$$

where $d$ is the spatial dimensionality of the system and $z$ is the dynamic scaling exponent. For a LNSM-CDW quantum phase transition in three dimensions $d = 3$ and $z = 1$ (exact results). On the other hand, in the large-N limit $\nu = 1$ and the fermionic anomalous dimension $\eta = 0$, yielding

$$\beta = \nu = 1. \tag{31}$$

Note that as we appraoch the quantum critical point, located at $V = V_c$, from either side of the transition the correlation length diverges as $\xi \sim \delta^{-\nu}$, implying $\delta \sim \xi^{-1/\nu}$. Therefore, using the scaling relations we find $m \sim \xi^{-\beta/\nu}$. Besides such leading power-law scaling, the dimensionless CDW OP is in general a function of another dimensionless

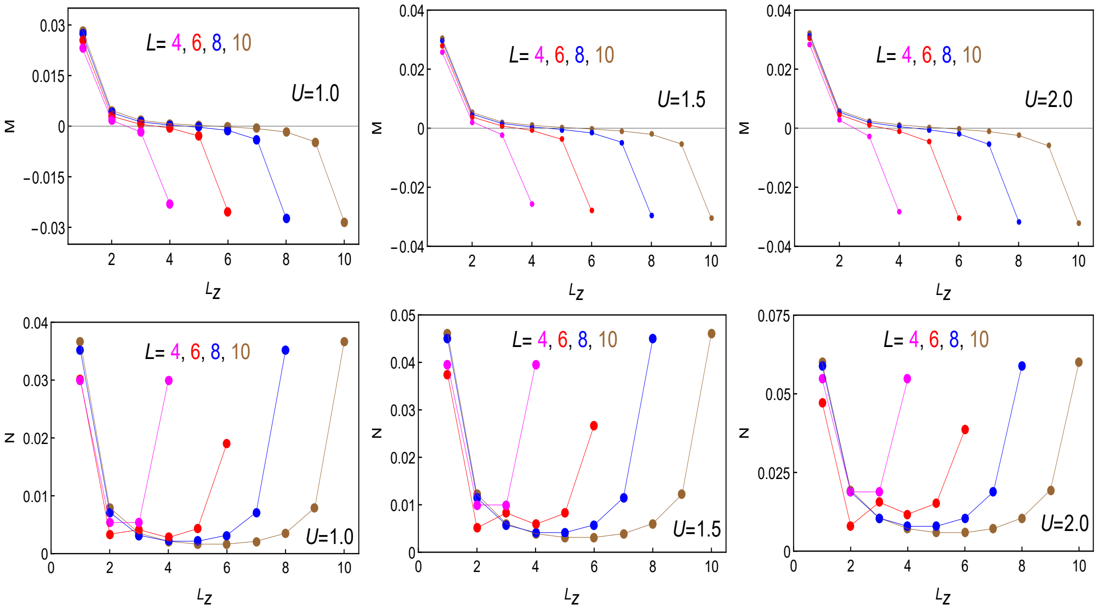


Figure 4: Spatial variation (along $z$ direction) of self consistent solution of ferromagnet ($M$) and antiferromagnet ($N$) order parameters for subcritical strength of onsite repulsion (quoted in each subfigure) are shown in upper and lower panels, respectively, in various systems of linear dimension $L$ (quoted in each subfigrue) along $z$ direction. Here $L_z$ is the layer index in the $z$-direction, along which we implement an open boundary.

variable $L/\xi$, where $L$ is the system size. Now applying general scaling argument we can arrive at the universal scaling of the CDW OP as

$$m = L^{-\beta/\nu} \, \mathcal{F}\left(\delta L^{1/\nu}\right) \quad \Rightarrow \quad mL^{\beta/\nu} = \mathcal{F}\left(L^{1/\nu}\left(V - V_c\right)\right), \tag{32}$$

where $\mathcal{F}$ is an universal, but in general an unknown function.

## IX. HARTREE-FOCK NUMERICAL ANALYSIS

We now present the details of Hartree-Fock analysis. First we focus on the nearest-neighbor (NN) interaction for which the interacting Hamiltonian reads as

$$H_{NN} = H_0 + \frac{V}{2} \sum_{\langle i,j \rangle} n_i n_j - \mu n, \tag{33}$$

where $\langle \cdots \rangle$ represents summation over NN sites, $n_i$ is the number operator at site $i$, $n$ is total number of electrons and $\mu$ is the chemical potential. For the sake of simplicity we here consider the femrions to be spinless. Here $H_0$ represents non-interacting system giving rise to a three dimensional LNSM [see Eq. (1)]. After usual Hartree decomposition we arrive at the following effective single-particle Hamiltonian

$$H^{SP}_{NN} = H_0 + V \sum_{\langle i,j \rangle} \left[ \langle n_{B,i} \rangle n_{A,j} + \langle n_{A,i} \rangle n_{B,j} \right] - \mu n, \tag{34}$$

where $n_{A(B)}$ counts the self-consistent site-dependent average electron density on sub-lattice $A(B)$. Since we always impose perdiodic boundary along $x$ and $y$ direction $n_{A/B}$ does not depend on $x$ and $y$. When we impose periodic boundary along $z$ direction, $n_{A/B}$ is uniform along $z$ direction as well, while it becomes a function of only $z$ co-ordinates or the layer index $L_z$ when we implement an open boundary in this direction. Let us measure these quantities relative to the uniform density at half-filling by defining

$$n_{A,i} = \frac{1}{2} + \delta_{A,i}, \; n_{B,i} = \frac{1}{2} - \delta_{B,i}. \tag{35}$$

The positive quantities $\delta_A$ and $\delta_B$ (function of position) determine the local CDW OP, with the constraint that system is always kept at half-filling

$$\sum_i \delta_{A,i} - \sum_i \delta_{B,i} = 0, \tag{36}$$

and we here choose $\mu = V/2$. The CDW OP ($m$) is then defined as

$$m = \frac{1}{2}\left(\delta_A + \delta_B\right), \tag{37}$$

and for brevity we here dropped the position dependence of all the quantities.

Next we turn our attention to onsite Hubbard repulsion. The interacting Hamiltonian in the presence of only onsite repulsion reads as

$$H_U = H_0 + U \sum_i n_{i,\uparrow} n_{i,\downarrow} - \mu n. \tag{38}$$

Once again we perform a Hartree decomposition to arrive at the following effective single-particle Hamiltonian

$$H_U^{SP} = H_0 + \sum_i \left[\langle n_{i,\uparrow}\rangle n_{i,\downarrow} + \langle n_{i,\downarrow}\rangle n_{i,\uparrow}\right] - \mu n. \tag{39}$$

We can write $n_{i,\sigma}$ as

$$n_{A,i,\sigma} = \frac{1}{2} + \sigma \delta_{A,i,\sigma},\; n_{B,i,\sigma} = \frac{1}{2} - \sigma \delta_{B,i,\sigma}, \tag{40}$$

where $\sigma = (+,-)$ corresponds to the spin projection $\uparrow, \downarrow$, respectively, and all quantities in the above equation are in principle position dependent. The constraint of half-filling is then maintained by choosing $\mu = U$ and

$$\sum_i \sum_{\sigma=\pm} \sigma \delta_{A,i,\sigma} - \sum_i \sum_{\sigma=\pm} \sigma \delta_{B,i,\sigma} = 0. \tag{41}$$

In this notation the local ferromagnet and anti-ferromagnet orders are defined as

$$M = \frac{1}{2}\left[\delta_{A,\uparrow} + \delta_{A,\downarrow} - \delta_{B,\uparrow} - \delta_{B,\downarrow}\right]; \quad N = \frac{1}{2}\left[\delta_{A,\uparrow} + \delta_{A,\downarrow} + \delta_{B,\uparrow} + \delta_{B,\downarrow}\right], \tag{42}$$

respectively. When we impose periodic boundary in all three directions then $M$ and $N$ are position independent, while they depend on the layer index in the $z$ direction when we implement open boundary in this direction.

---

[1] H. B. Nielsen and M. Ninomiya, Nucl. Phys. **185**, 20 (1981).
[2] I. F. Herbut, Phys. Rev. B **83**, 245445 (2011).
[3] T. Senthil, and R. Shankar, Phys. Rev. Lett. **102**, 046406 (2009).
[4] Co-dimension $d_c$= physical dimension ($d$) - dimensionality of the hyperplane over which energy gap vanishes. Hence, for a $d$-dimensional Fermi surface $d_c = d - (d-1) = 1$ and for a Fermi point system $d_c = d - 0 = d$. For a three dimensional LNSM $d_c = d - 1 = 2$.
[5] J. A. Gracey, Int. J. Mod. Phys. A **9**, 727 (1994).
[6] L. Rosa, P. Vitale, and C. Wetterich, Phys. Rev. Lett. **86** 958 (2001); F. Höfling and C. Nowak, and C. Wetterich, Phys. Rev. B **66**, 205111 (2002).
[7] I. F. Herbut, Phys. Rev. B **85**, 085304 (2012).
[8] S. Okubo, J. Math. Phys. **32**, 1657 (1991).
[9] P. Goswami, and A. H. Nevidomskyy, Phys. Rev. B **92**, 214504 (2015).
[10] S. Bera, J. D. Sau, and B. Roy, Phys. Rev. B **93**, 201302(R) (2016).
